# Supplementary material for: Robust Quantum Control via Multipath Interference for Thousandfold Phase Amplification in a Resonant Atom Interferometer
Source: arXiv:2407.11246 ancillary file (2024-12-12)
Supplement: Supplementary file 1 [file Resonant_AI_Supplement.pdf]

# Supplemental Material for "Robust Quantum Control via Multipath Interference for Thousandfold Phase Amplification in a Resonant Atom Interferometer"

Yiping Wang*,[1] Jonah Glick*,[1] Tejas Deshpande*,[1] Kenneth DeRose*,[1] Sharika Saraf,[1] Natasha Sachdeva,[1,2] Kefeng Jiang,[1] Zilin Chen,[1] and Tim Kovachy[1,†]

[1]*Department of Physics and Astronomy and Center for Fundamental Physics, Northwestern University*
[2]*Q-CTRL, Quantum Applications and Algorithms Division*

This Supplemental Material provides further details on the following topics: the experimental apparatus (Sec. I), the semi-classical model and optimization algorithms used for open-loop optimization (Sec. II), the preservation of the benefits of optimization as the interferometer pulse spacing is increased (Sec. III), the theoretical form of the resonant atom interferometer response function vs. frequency (Sec. IV), the optical Bloch equation simulator used to model the effects of spontaneous emission (Sec. V), the gradient ascent algorithm used for closed-loop optimization (Sec. VI), and Bloch sphere visualization and supplementary simulations pertaining to the emergence of a cumulative phase from spontaneous emission (Sec. VII).

## I. APPARATUS

We perform interferometry on a cloud of $^{88}$Sr atoms using the 689 nm $^1S_0$-$^3P_1$ intercombination line. The atoms are released from a magneto-optical trap (MOT) operating on the 461 nm $^1S_0$-$^1P_1$ transition. A cold beam of Sr atoms is delivered to the science chamber by an AOSense Sr atom source and 461 nm light from external laser systems. Anti-Helmholtz coils produce magnetic field gradients (55 G/cm along the axis of the coils), while 461 nm beams and repumper beams at 679 nm and 707 nm create a 3D MOT. The frequency of the 461 nm beams is locked to the $^1S_0$-$^1P_1$ transition via an absorption lock aligned through the atom source's oven viewports.

The 689 nm interferometer beam, generated by an M-Squared SolsTis pumped by an 18 W Equinox 532 nm laser, targets the $^1S_0$-$^3P_1$ transition and is referenced via a beatnote lock to a 689 nm reference beam stabilized to a Stable Laser Systems ultra-low expansion (ULE) cavity. Figure 1 shows the orientations of the interferometer and state-selective push beams relative to the 3D MOT chamber. The interferometer beam propagates through an acousto-optic modulator (AOM) from AA Opto-Electronic (MQ180-A0,25-VIS) in a single-pass configuration. This AOM serves as the actuator for pulse amplitude and phase. The first diffracted order is coupled into a single-mode, polarization-maintaining fiber, which delivers 1.2 W of power to the atoms. A bias field of $\approx$ 9.5 Gauss is applied to set the quantization axis of the atoms and shift the $m_j = \pm 1$ Zeeman sublevels of the $^3P_1$ state far enough away from the $m_j = 0$ transition relative to the nominal Rabi frequency so that under an imperfect interferometer beam polarization, population lost to these sublevels during an interferometric sequence is suppressed. We align the polarization of the laser beam to be parallel to the bias field.

After the interferometer pulse sequence, $\approx$ 80 mW of blue light is directed on the atom cloud for $\approx 5\ \mu$s to push the atom population that is in the $^1S_0$ state away from the atoms in the $^3P_1$ state. We wait $\approx$ 5 ms during which time the pushed $^1S_0$ population spatially separates from the $^3P_1$ population, and the $^3P_1$ population decays to the $^1S_0$ state. Both clouds are then fluoresced by counter-propagating blue light for 500 $\mu$s. The resulting image is of two clouds—a pushed cloud that consists of atoms that compose the 'ground state' output port of the interferometer and an unpushed cloud that forms of the 'excited state' output port of the interferometer. The population in each output port is extracted by summing over the rows of the resulting fluorescence image and fitting the resulting plots to a sum of two Gaussian functions [1]. A timing system which includes an M-Labs ARTIQ system controls the timings associated with the release of atoms from the MOT, the interferometer beam pulse durations and phases, and the imaging of the atoms.

## II. OPEN-LOOP OPTIMIZATION – SEMI-CLASSICAL STRAY TRAJECTORY CALCULATOR

In this section, we will discuss three topics: 1. The semi-classical model used to compute the population in different interferometer paths under imperfect mirror pulse operations. 2. The construction of a cost function based on these

† timothy.kovachy@northwestern.edu

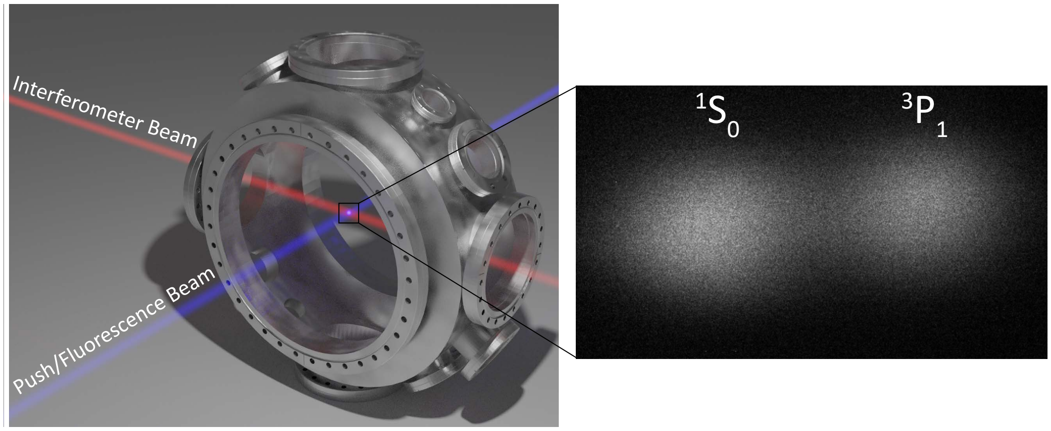


FIG. 1. The science chamber with the orientations of the interferometer and push/fluorescence beams. A camera is used to capture an image of the fluoresced atom clouds that correspond to the two atom energy states, from which we extract information about interferometer visbility and phase.

theoretically determined populations, along with methods for determining optimal laser phases which minimize the cost function and result in an interferometer more robust to $\pi$-pulse infidelity. 3. A cost-function-driven explanation as to why the UR-N [2] pulse sequences, which work well for dynamically decoupling qubit systems from their environment, lose signal sensitivity when applied to resonant atom interferometers.

### A. The Semi-Classical Model

We outline the traditional semi-classical approach and show that for our application, the calculation can be significantly simplified. The traditional semi-classical approach to compute phase shifts in atom interferometry [3, 4] is to associate a 'propagation' phase $\phi_{\text{prop}}$ and 'laser' phase $\phi_{\text{laser}}$ with individual trajectories. Assuming the interferometer beam is oriented along the $x$-axis, and considering a system in one spatial dimension where any two arms are separated in momentum space by a single photon recoil momentum ($\hbar k$), these two phases can be expressed as

$$\phi_{\text{prop}} = \frac{1}{\hbar}\int_{t_i}^{t_f} dt(L[x_{\text{cl}}[t]] - E[t])$$
$$\phi_{\text{laser}} = \sum_{j=1}^{n}(-1)^{j+1}(k\, x_{\text{cl}}[t_j] + \phi_L[t_j])$$

where $\phi_L[t]$ is the overall phase of the interferometer beam at time $t$, $k$ is the wavenumber of the interferometer beam, and the $n$ kicks occur at times $t_j$, where $j = 1, 2, ..., n$. $E[t]$ is the internal energy of the trajectory at time $t$, and $x_{\text{cl}}[t]$ is the classical path of this trajectory. We take $t_i$ to be a time prior to the first beamsplitter pulse, and time $t_f$ to be a 'final' time where $t_f > t_n$. The propagation phase is the phase accumulated by a trajectory $x_{\text{cl}}[t]$ between laser pulses, proportional to the action $S$ associated with that trajectory. The laser phase is associated with the imprint of the phase of the laser onto the phase of the trajectory. To compute phase differences between two trajectories, we take the difference of the sum of their laser and propagation phases, then add on a 'separation' phase $\Delta\phi_{\text{sep}}$ associated with the spatial separation of two trajectories which compose one interferometer output port.

$$\Delta\phi_{\text{prop}} = \phi_{\text{prop}}^{\text{upper}} - \phi_{\text{prop}}^{\text{lower}}$$
$$\Delta\phi_{\text{laser}} = \phi_{\text{laser}}^{\text{upper}} - \phi_{\text{laser}}^{\text{lower}}$$
$$\Delta\phi_{\text{sep}} = -\frac{m}{2\hbar}(\dot{x}_{\text{cl}}^{\text{upper}}[t_f] + \dot{x}_{\text{cl}}^{\text{lower}}[t_f])(x_{\text{cl}}^{\text{upper}}[t_f] - x_{\text{cl}}^{\text{lower}}[t_f])$$

so that the overall phase shift between two trajectories can be expressed as $\Delta\phi = \Delta\phi_{\text{prop}} + \Delta\phi_{\text{laser}} + \Delta\phi_{\text{sep}}$.

### 1. The Laser Phase For Single-Photon Transitions

The laser phase $\phi_{\text{laser}}$ in the semi-classical approach [3, 4] is based on interferometers whose atom-optics operations are achieved by counter-propagating two-photon transitions, like Bragg or Raman transitions. For single-photon transitions, we can associate a similar phase to each atom-light interaction. This can be thought of as emerging from the finite light travel time of the interferometer beam from the laser to the atoms [5]. We will now make the case for this in a way that is consistent with stray paths. If the laser is located at position $x = 0$, and the photons travel immediately to the classical trajectory, then the phase accumulated by the trajectory from time $t_i$ to time $t_f$ under just its internal energy would be

$$\phi_{\text{internal, no travel time}} = \sum_{j=1}^{n}(-1)^{j+1}\omega_A t_j + \begin{cases} 0, & n \text{ even} \\ -\omega_A t_f, & n \text{ odd} \end{cases}$$

where we take the ground state energy to be zero, and the resonant frequency of the atomic transition to be $\omega_A$. If we now consider the finite light speed $c$, then the time it takes to reach the trajectory is $x_{\text{cl}}[t_j]/c$. We assume that the trajectory's position does not change between the time the photon is emitted $t_j$ and the time the photon reaches the atom under the assumption that the velocity of the atom is small compared to the speed of light. In this case, a pulse emitted at time $t_j$ will not reach the atom until time $t_j + \frac{x_{\text{cl}}[t_j]}{c}$ so that the total accumulated internal phase associated with a trajectory is

$$\begin{aligned} \phi_{\text{internal}} &= \sum_{j=1}^{n}(-1)^{j+1}\omega_A \Big(t_j + \frac{x_{\text{cl}}[t_j]}{c}\Big) + \begin{cases} 0, & n \text{ even} \\ -\omega_A t_f, & n \text{ odd} \end{cases} \\ &= \phi_{\text{internal, no travel time}} + \sum_{j=1}^{n}(-1)^{j+1}\frac{\omega_A}{c}x_{\text{cl}}[t_j] \end{aligned}$$

When the light is resonant with the atomic transition, $k = \omega_A/c$ so that the second term in this expression becomes

$$\sum_{j=1}^{n}(-1)^{j+1}k\, x_{\text{cl}}[t_j]$$

which is the same term that emerges from the traditional semi-classical approach to the laser phase accumulated under two-photon transitions. For convenience, we group this contribution into what we call the laser phase.

### 2. Simplifying the Calculation

For the systems we consider in this paper, many of the terms which contribute to the phase shift cancel and do not need to be computed, substantially simplifying the model, even if the trajectories are stray trajectories spawned by imperfect atom-optics operations. In the model, we assume that non-overlapping paths do not interfere so that the benefits of optimization are independent of the pulse spacing. This assumption corresponds to the 'short coherence length' limit, where trajectories in the same internal state and which move with the same external center-of-mass velocity do not interfere if displaced slightly. For the interferometer to be resonant with lower frequency signals, the time between mirror pulses must increase, which also increases the distance between stray and main trajectories. By assuming that atom-light interaction points are spaced beyond a coherence length, the optimization generates pulse sequences that remain effective even as these distances vary (see Sec. III). The separation phase scales with the separation between two trajectories. Under the assumption described above, any trajectories that interfere with each will overlap perfectly, so by definition the separation phase will be zero.

Consider a Lagrangian given by

$$L = \frac{m}{2}\dot{x}^2 + ma[t]x$$

where $a[t]$ is a time dependent acceleration and forces that vary across the wavefunction are assumed to be small (no higher order terms in $x$). We can perform a Galilean transformation to a new frame with Lagrangian

$$L = \frac{m}{2}\dot{x}^2$$

where the influence of $a[t]$ in the original frame is transformed into the laser phase $\phi[t]$ [3, 6]. For the purpose of the optimizer, we do not include the $a[t]$ dependent laser phase in the transformed system, but it could correspond to a signal to be measured.

Consider an atom in the ground internal state located at position $x_i$ at time $t_i$ and moving with a velocity $v_x$. Under subsequent imperfect atom-optics operations, a number of 'kicks' are imparted onto the trajectory. Consider one such trajectory which is kicked a total of $n$ times over the course of the interferometer cycle, with kicks occurring at time $t_j$, where $j = 1, 2, 3, ..., n$. $n$ could vary depending on the number of loops in the cycle and the number of missed kicks for a particular trajectory. The classical path such a trajectory takes can be written as

$$x_{\mathrm{cl}}[t] = x_i + v_x(t - t_i) + v_r \sum_{j=1}^{n} (-1)^{j+1}(t - t_j)\Theta[t - t_j] \tag{1}$$

where $v_r$ is the 'recoil' velocity, $t_k$ is the time of the $k^{\mathrm{th}}$ kick, $t_i < t_1$, and $\Theta$ is the Heaviside step function. The factor of $(-1)^k$ comes from the fact that the first kick—which corresponds to the absorption of the a photon—will kick the trajectory in the $+x$ direction, and the next kick—which corresponds to stimulated emission—will kick the trajectory in the $-x$ direction. At a 'final' time, $t_f > t_n$, after all the atom-optics operations are performed, the final position of the trajectory, $x_f$, can be written using Eq. 1 as

$$x_f = x_i + v_x(t_f - t_i) + v_r\tau + \begin{cases} 0, & n \text{ even} \\ v_r t_f, & n \text{ odd} \end{cases} \tag{2}$$

where

$$\tau = \sum_{j=1}^{n} (-1)^j t_j \tag{3}$$

carries all the dependence on the kick times $t_j$. The key point is that using Eq. 2, we can write $\tau$ purely in terms of variables that are the same for two closed trajectories: The initial space-time coordinate of the atom $(x_i, t_i)$, the final space-time point of the trajectory $(x_f, t_f)$, $v_x$, and $v_r$:

$$\tau = \frac{1}{v_r}\left( x_f - x_i - v_x(t_f - t_i) - \begin{cases} 0, & n \text{ even} \\ v_r t_f, & n \text{ odd} \end{cases} \right)$$

Any two closed trajectories will also have the same value of $n$ mod 2 because they are in the same internal state, so the value of $\tau$ will be the same for both trajectories, regardless of the specific values of $t_j$. We will now prove that the propagation phase and the component of the laser phase that depends on the classical trajectory can also both be expressed in terms of $\tau$ for an individual trajectory, without any other explicit dependence on $t_j$, and therefore cancel between any two closed trajectories. The propagation phase associated with a trajectory in the semi-classical limit can be written as

$$\phi_{\mathrm{prop}} = \frac{1}{\hbar}\int_{t_i}^{t_f} dt \frac{m}{2}(\dot{x}_{\mathrm{cl}}[t])^2 - \frac{1}{\hbar}\int_{t_i}^{t_f} dt E[t]$$

Using Eq. 1, we can write

$$\begin{aligned} \phi_{\mathrm{prop}} =& \frac{m}{2\hbar}\left( v_x^2(t_f - t_i) + (v_r^2 + 2v_r v_x)\left( \tau + \begin{cases} 0, & n \text{ even} \\ t_f, & n \text{ odd} \end{cases} \right) \right) \\ & - \tau\omega_A + \begin{cases} 0, & n \text{ even} \\ -\omega_A t_f, & n \text{ odd} \end{cases} \end{aligned}$$

Therefore, the propagation phase cancels between any two trajectories which form a closed loop.

Here we make the argument that the term that is proportional to $kx_{\text{cl}}[t]$ in the laser phase cancels between trajectories that form closed loops. Using Eq. 1, we can write this component as

$$\sum_{j=1}^{n}(-1)^{j+1}(kx_{\text{cl}}[t_j]) = k\begin{cases}(v_r+v_x)(-\tau), & n \text{ even}\\ x_i - v_x t_i + v_x(-\tau), & n \text{ odd}\end{cases}$$

This contribution to the laser phase also depends on parameters that are equal for trajectories that form closed loops and will cancel between them.

### 3. *Computing Trajectory Populations*

Under a semi-classical approximation, we associate the quantum state of the atom with a superposition of classical trajectories. The populations in each trajectory are computed in the following way: First, a beamsplitter pulse splits the atom wavefunction $|\Psi\rangle$ at time $t_1$ into a superposition of a 'kicked' state and an 'unkicked' state

$$|\Psi\rangle = \frac{1}{\sqrt{2}}|{}^1S_0, x[t_1]\rangle + \frac{-i}{\sqrt{2}}|{}^3P_1, x[t_1]\rangle$$

where the two states are written as $|\text{internal state, associated classical position}\rangle$. A subsequent mirror pulse is performed wherein the total number of trajectories is doubled, with 2 trajectories being stray paths corresponding to population that did not receive a kick by the mirror pulse operation, and the other two paths composing the main interferometer arms corresponding to efficiently kicked atom population. The mirror pulse at time $t_j$ is taken to perform the operation

$$|{}^1S_0, x[t_j]\rangle \to \sqrt{f}|{}^1S_0, x[t_j]\rangle + -i\sqrt{p}e^{i\phi}|{}^3P_1, x[t_j]\rangle$$
$$|{}^3P_1, x[t_j]\rangle \to -i\sqrt{p}e^{-i\phi}|{}^1S_0, x[t_j]\rangle + \sqrt{f}|{}^3P_1, x[t_j]\rangle$$

on each trajectory, where $x[t_j]$ is the position of the trajectory at the pulse time $t_j$, $p$ is the fraction of the population in this trajectory that is successfully kicked, and whose phase is shifted by the phase of the laser ($\phi$), and $f$ is the fraction of the population in this trajectory that fails to be kicked, so that $p+f=1$. The first two mirror pulses do not result in interference of any stray trajectories. However, starting with the third mirror pulse and continuing thereafter, an additional computational step is introduced to capture the fact that stray trajectories in the same internal state and position will spatially overlap and interfere. To account for this, after performing the mirror pulse operation indicated above, we check for such interfering trajectories and merge them such that a trajectory with population $P_1$ and phase $\phi_1$ which is overlapping with a trajectory with population $P_2$ and phase $\phi_2$ becomes a single trajectory with population $P_3$ and phase $\phi_3$, where

$$\sqrt{P_3}e^{i\phi_3} = \sqrt{P_1}e^{i\phi_1} + \sqrt{P_2}e^{i\phi_2}$$

$$P_3 = P_1 + P_2 + 2\sqrt{P_1P_2}\cos[\phi_1 - \phi_2]$$
$$\phi_3 = \text{arctan2}[\sqrt{P_1}\sin[\phi_1] + \sqrt{P_2}\sin[\phi_2], \sqrt{P_1}\cos[\phi_1] + \sqrt{P_2}\cos[\phi_2]]$$

where $\text{arctan2}[x_1, x_2]$ is the angle between the positive $x$ axis and the line that is made from the origin to the point $(x_2, x_1)$. We ignore the contribution of the term that is proportional to $kx_{\text{cl}}[t]$ in the laser phase, the propagation phase, and the separation phase as discussed in Sec. II A 2.

Applying these operators at each mirror pulse time, and allowing trajectories to propagate freely in between mirror pulses, results in a spatial spread of atom populations whose structure depends on the choice of mirror pulse laser phases. At the time exactly in the middle of two mirror pulses, all trajectories naturally group into families of trajectories (see Fig. 2), with the *central* family comprising the two main arms of the interferometer and their re-entered stray paths. We define the population of a 'family' of trajectories to be equal to the sum of the population of the trajectories that compose it. We define the central family population after the $m^{\text{th}}$ mirror pulse operation as $F_{0,m}$. The population of a family that is $n$ families away from the central family after the $m^{\text{th}}$ mirror pulse operation is written as $F_{n,m}$, so that the index $n$ denotes a discretized spatial coordinate associated with the position of the family of trajectories and $m$ denotes a discretized temporal coordinate.

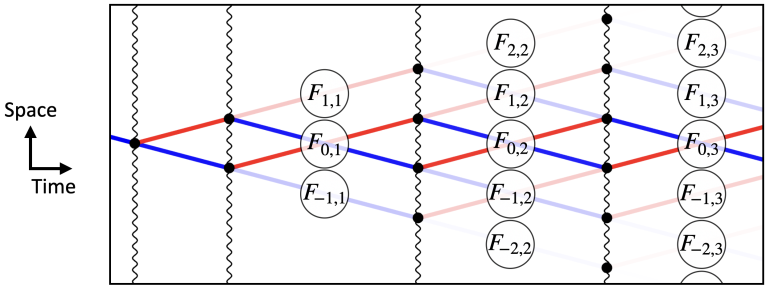


FIG. 2. Definition of *family population* $F_{n,m}$. Notice the interference of stray paths does not occur until the third mirror pulse operation.

### B. How the Cost Function is Defined and the Phase Optimization is Done

Different stray paths correspond to different 'missed' laser pulses and will therefore accumulate different laser phases. Paths which contribute to families far from the central family (large $n$) will carry less phase information about the oscillating signal owing to the fewer imprinted phases from the laser onto the trajectory. We construct a cost function for which population at or near the central interferometer arms is preferred, and population far from the central families is penalized. We find this cost function to result in large fringe visibility and phase sensitivity to resonantly oscillating laser phases in the interferometer. The cost function $J$ is given by

$$J[\phi_1, \phi_2, ...\phi_N] = \sum_{m=3}^{L} \sum_{n=-m}^{m} F_{n,m} n^2 \tag{4}$$

where the population of any family contributes to the cost proportional to the square of its distance from the central family ($n^2$), and a temporal average of the population spread is performed. The reason for the temporal index started at $m = 3$ is that prior to the 3$^{\text{rd}}$ laser pulse, no stray trajectories overlap, and so the population in families prior to that pulse are completely independent of the phases of the mirror pulse operations. After the $m^{\text{th}}$ pulse, there are a total of $2m + 1$ families, and the sum over the discretized spatial coordinate runs from $-m$ to $m$.

In the language of this calculator, an explanation of the resonant enhancement seen in the laboratory (see Fig. 2(d) of the main text) is that stray paths which contribute to families far from the central family destructively interfere with one another through the differently accumulated laser phases, whereas the stray trajectories that are re-directed and re-enter the central family constructively interfere and enhance the overall sensitivity to the oscillating laser phase.

The $N$-dimensional optimization problem consists of determining $N$ laser phases in such a way that the cost $J$ is minimized. In general, the cost function $J$ has nontrivial, and non-convex, dependence on the mirror pulse phases. We find that the overall phase of the sequence has little impact on interferometer performance, so we constrain the first laser phase to be zero to reduce the dimensionality of the problem to $N - 1$. We then optimize the cost function by exploring the $N - 1$ dimensional space of possible laser phases. Initially, we perform grid sampling for $N = 8$, evaluating the cost for laser phases sampled evenly between 0 and $2\pi - a_\phi$, with a spacing of $a_\phi$. This creates a lattice of evenly spaced points in the $N - 1$-dimensional space of possible phases. We find that for $a_\phi = \pi/4$, some of the top-performing sequences have a mirror symmetry so that their phase patterns have the form $(\phi_1, \phi_2, \phi_3, \phi_4, \phi_4, \phi_3, \phi_2, \phi_1)$. This mirror symmetry constraint has the additional benefit of reducing the dimensionality of the optimization problem to $N/2 - 1$, which reduces the computational complexity of the optimization. We therefore impose this symmetry for further refining the optimization per the methods discussed below. In future work, higher dimensional optimizations without this constraint could be further explored.

After this initial evaluation, we refine our search using two methods: gradient descent and Bayesian optimization. For the gradient descent optimization, we use the initially sampled grid points as initial guesses and perform gradient descent numerically starting from each point in the lattice. The cost function is computed over $L = 64$ loops. For the Bayesian optimization, we use the initial grid points to populate the initial Gaussian Process (GP) model using a squared exponential kernel [7]. Each grid point provides an initial set of observations for the GP, which is used to build a surrogate model of the cost function. We perform 100 steps of Bayesian optimization, where each new point in the 3D space is selected based on the maximum of the 'expected improvement' acquisition function. The optimization routines are executed in a Mathematica script, and call a C++-based cost function calculator operating on the semi-classical model. It happens that for this problem, neither gradient descent nor Bayesian optimization

yield sequences that minimize the cost better than those identified by the initial grid sampling. We find that the two sequences which minimize the cost for $L = 64$ are $(0, \frac{\pi}{2}, \frac{3\pi}{2}, \pi, \pi, \frac{3\pi}{2}, \frac{\pi}{2}, 0)$ and $(0, \frac{3\pi}{2}, \frac{\pi}{2}, \pi, \pi, \frac{\pi}{2}, \frac{3\pi}{2}, 0)$. In the main text, we take the first of these two sequences and add an overall phase of $+3\pi/8$ to each of the phases in the sequence, though we note that the overall phase offset does not significantly impact the performance of the interferometer.

For the $N = 16$ problem, we impose the same constraints as discussed above to reduce the dimensionality of the problem to 7. We perform a grid sampling with spacing $a_\phi = \pi/2$ for a total of $4^7 = 16,384$ evaluated points, running the cost function for $L = 64$, as we did for the $N = 8$ case. We find that one of the optimal sequences which emerges from this grid sampling is of the form $(0, \pi, \frac{3\pi}{2}, \pi, \frac{3\pi}{2}, \frac{\pi}{2}, 0, \frac{\pi}{2}, \frac{\pi}{2}, 0, \frac{\pi}{2}, \frac{3\pi}{2}, \pi, \frac{3\pi}{2}, \pi, 0)$. Running this sequence in the laboratory produces an interferometer with a visibility of $(6.0 \pm 0.2)\%$ at $L = 496$. The optimal $N = 8$ sequence at $L = 496$ produces an interferometer with a visibility of $(4.1 \pm 0.5)\%$, corresponding to an $\approx 1.5$x increase in the visibility of the interferometer associated with extending from $N = 8$ to $N = 16$. Here the uncertainty in the visibility comes from the uncertainty of the sinusoidal fit to the interference fringe. As in the $N = 8$ case, it happens that for this $N = 16$ optimization problem, the best sequences for cost function minimization come from initial grid sampling, and that subsequently applying gradient descent using the grid points as initial guesses does not yield improved sequences.

One benefit of this open-loop approach to searching for laser phases which maximize interferometer visibility and phase sensitivity at high loop number, despite losing population to stray paths, is that a simulation of an experiment cycle can run more quickly than the duty cycle of the real experiment ($\sim 10$ ms vs. $\sim 10$ s to scan a fringe). The $N$-dimensional optimization problem requires many evaluations of the cost function, so a speedy evaluation can enable optimization for larger $N$. A detriment of open-loop optimization in general is that the model might not account for relevant physical phenomena in a cost function which the closed-loop approach would capture. As shown in the main text, we find that the closed-loop optimization converges to similar results as our open-loop optimization.

### C. $UR{-}N$ Sequences Applied To Atom Interferometry

We observe that the UR-L sequences mentioned in the main text [2] enhance the total population in the central family after the last mirror pulse in an $L$-loop sequence, $F_{0,L}$. This comes at the expense of permitting a large spread in trajectories during the cycle, which renders the phase of the interferometer less sensitive to resonantly oscillating signals (see Fig. 4). This large spread in the trajectories is associated with a large cost in Eq. 4, owing to the $n^2$ dependence, so that at large $L$, the UR-L sequences are out-performed by other sequences. We find that when optimizing over a large number of pulses, incorporating the spatial spread of all stray trajectories into a cost function results in sequences which maximize fringe visibility and leave the phase response of the interferometer sensitive to oscillating signals. Figure 3 compares the spread of trajectories associated with the $UR-16$ sequence vs. the cost-function-optimizated $N = 16$ sequence for a 64 loop interferometer sequence. The cost-function-optimized sequence does a better job of keeping the spatial spread of atom population close to the central family trajectories throughout the interferometer, whereas the $UR-16$ sequence produces a larger spread. Figure 4 demonstrates the fall-off in the sensitivity of a multi-loop atom interferometer operating on the $UR-N$ sequence as a function of $N$. As $N$ is increased, keeping $L$ constant and repeating the $N$-pulse sequences $L/N$ times to compose the $L$-loop sequence, we find that the phase response of the interferometer to resonantly oscillating signals is suppressed. We associate this suppression with the increased spread in the population of stray trajectories in the $UR-N$ sequence as $N$ increases.

## III. EFFECT OF INCREASING PULSE SPACING

In this section, we present data showing that the benefits of optimization are retained as the mirror pulse spacing is increased so that neighboring families of trajectories (see Fig. 2) are spaced by more than a coherence length. This indicates that—as expected from how we structure our optimization approach (see Sec. II)—the optimized sequences do not rely on interference across different families.

Figure 5(a) presents a measurement of the atomic coherence length in our system. We run an asymmetric Mach-Zehnder sequence, where the final beamsplitter time is offset by $\delta T$, for a range of different values of $\delta T$. The measured visibility is plotted versus arm separation, $\delta d_a = v_r \times \delta T$, at the time of the final beamsplitter, depicted in the inset. The shaded areas in both plots denote regions within the coherence length of $x_c = 2.39 \pm 0.14$ nm, defined by the equation $V(\delta d_a) = V(0)\exp(-\frac{2\delta d_a^2}{x_c^2})$, which is 4 times the coherence length defined in [8]. Our definition of coherence length corresponds to a $1/e^2$ decay in visibility when the arms are separated by a coherence length.

Figure 5(b) illustrates the decay in visibility as a function of the distance between neighboring families of trajectories (i.e., the distance between neighboring atom-laser interaction points, where different sets of trajectories converge),

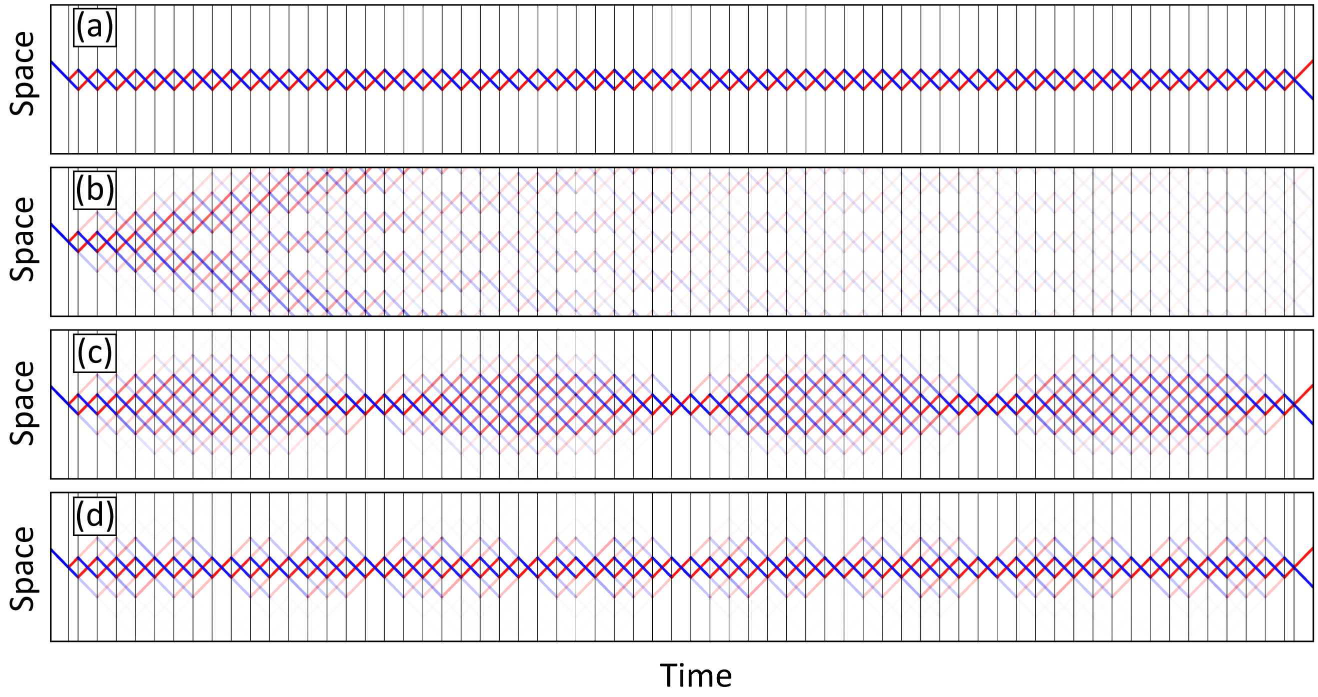


FIG. 3. Comparison of trajectory populations for a 64 loop interferometer sequence with (a) perfect mirror pulse operations, (b) imperfect mirror operations and no phase modulation, (c) a UR-16 sequence repeated 4 times, and (d) a cost-function-optimized $N = 16$ sequence repeated 4 times. The spread of the population into trajectories far from the central two interferometer arms in the case of the repeated UR-16 sequence results in reduced sensitivity of the interferometer phase to resonantly oscillating signals. The 16 laser phases of this UR-16 sequence are $(0, \frac{7\pi}{4}, \frac{5\pi}{4}, \frac{\pi}{2}, \frac{3\pi}{2}, \frac{\pi}{4}, \frac{3\pi}{4}, \pi, \pi, \frac{3\pi}{4}, \frac{\pi}{4}, \frac{3\pi}{2}, \frac{\pi}{2}, \frac{5\pi}{4}, \frac{7\pi}{4}, 0)$. The 16 laser phases of the cost-function-optimized $N = 16$ sequence are $(0, \pi, \frac{3\pi}{2}, \pi, \frac{3\pi}{2}, \frac{\pi}{2}, 0, \frac{\pi}{2}, \frac{\pi}{2}, 0, \frac{\pi}{2}, \frac{3\pi}{2}, \pi, \frac{3\pi}{2}, \pi, 0)$.

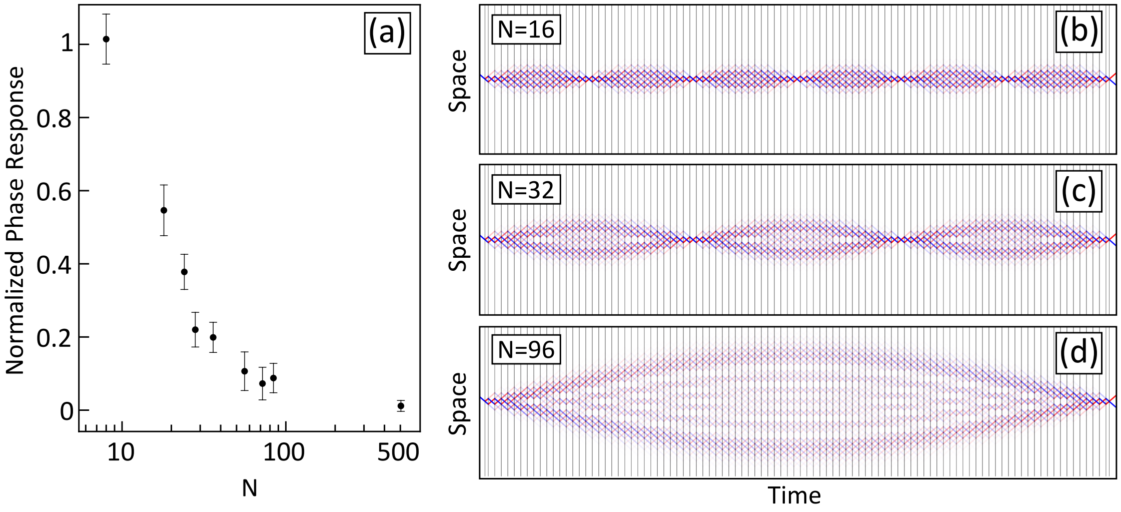


FIG. 4. Comparison of UR-N sequences for different values of $N$. (a) Experimentally determined phase sensitivities for different values of $N$ for a 504 loop sequence. The normalized phase response is defined to be $(\Delta\phi[\delta\phi = \pi/(504 \times 2)] - \Delta\phi[\delta\phi = 0])/\pi$, where $\Delta\phi$ is the measured interferometer phase, and $\delta\phi$ is the amplitude of the resonantly modulating phase. The error bars come from uncertainties in the sinusoidal fits to the interference fringes. Panels (b), (c), and (d) show the spatial spread in atom population for $N = 16$, $N = 32$, and $N = 96$ respectively for a 96 loop interferometer sequence, as determined by the semi-classical model.

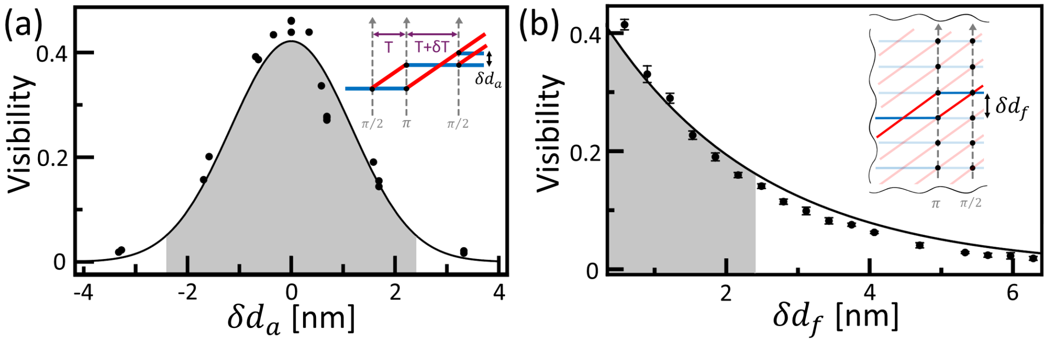


FIG. 5. (a) Visibility of an asymmetric Mach-Zehnder sequence (inset) as a function of the separation between the two arms at the final beamsplitter. The solid black dots are measured data, and the curve is the result of a fit to the data. (b) Visibility decay in an optimized sequence over 64 loops, plotted as a function of the distance between neighboring atom-laser interaction points (where different sets of trajectories converge, shown in the inset). The solid black dots are measured data. A solid line on the graph represents the theoretically expected visibility decay due to spontaneous emission, highlighting the fundamental limitations on visibility. Error bars indicate the standard error from the fitting of interference fringes. The shaded areas on both graphs denote regions within the coherence length.

$\delta d_f = v_r \times \left(\frac{\tau_m}{2} + \tau_{\frac{\pi}{2}}\right)$, in a 64-loop interferometer sequence operating on the optimized $N = 8$ set of laser phases. $\tau_m$ represents the deadtime between mirror pulses, and $\tau_{\frac{\pi}{2}}$ is the duration of the beamsplitter pulses. As $\tau_m$ is increased, the deadtime between a beamsplitter pulse and the nearest mirror pulse, $\tau_b$, scales as $\tau_b = \frac{1}{2}(\tau_m - \tau_{\frac{\pi}{2}})$, which we found maximizes fringe visibility. The results demonstrate that increasing the pulse spacing—and thus extending the distance between neighboring families beyond a coherence length—preserves the benefits of the optimization. Namely, the observed decline in visibility as $\tau_m$ increases aligns with the anticipated scaling of visibility loss due to spontaneous emission over longer sequence durations (detailed in Sec. VII). No further degradation is evident with increasing $\tau_m$.

## IV. RESONANT INTERFEROMETER RESPONSE FUNCTION

In Fig. 2(f) of the main text, we present measurement results of the resonant interferometer response of our optimized sequence as a function of oscillating signal frequency, as well as its corresponding theory curve. We applied an oscillatory laser phase as our signal: $\delta\theta(t) = A_\theta \sin(\omega t)$, where $A_\theta$ is the amplitude of the oscillating phase and $\omega$ is its frequency. In an interferometer with even loop number $L$, under perfect atom-optics operations that occur instantaneously, the phase shift due to this oscillatory laser phase is $\Delta\phi = \delta\theta(0) + 2\sum_{j=0}^{L-1}(-1)^{j+1}\delta\theta(T + 2jT) - \delta\theta(2LT) = 2A_\theta \sin\left(\frac{\omega T}{2}\right)^2 \frac{\sin(2L\omega T)}{\cos(\omega T)}$. We assume the first beamsplitter occurs at time $t_0 = 0$, with time $T$ separating beamsplitter and mirror pulses and $2T$ separating mirror pulses. For large $L$, the response of the interferometer is resonant at $\omega_{\text{res}} = \frac{\pi}{2T}$. For the data shown in Fig. 2(f), we used $2T = 192$ ns for mirror pulses of 96 ns duration, with $2T$ corresponding to the spacing between the centers of subsequent pulses in the experiment. In the experiment, we apply laser phases in such a way that the phase of pulse $i$ is chosen to be equal to $\delta\theta(t_i)$ where $t_i$ is time at the center of the finite duration pulse. The measured phase response agrees closely with this theoretical response function, despite imperfect atom-optic interactions throughout the interferometer sequence.

## V. OPTICAL BLOCH EQUATION SIMULATIONS

### A. Details of the Simulator

For some of our studies, we perform simulations that incorporate the effects of spontaneous emission. For this purpose, it is convenient to simulate the interferometer in momentum space, so that we solve for the dynamics of the coupled states $|^1S_0, p\rangle$ and $|^3P_1, p + \hbar k\rangle$ and then integrate over a distribution of momenta $p$. For each $p$, we solve the optical Bloch equations (OBE) to determine the time evolution of the density matrix for an atom which starts in the ground state and which is subject to the laser pulses associated with an interferometer sequence. We assume an interferometer beam with a Gaussian profile and radial beam waist $w_0$ ($1/e^2$ of the intensity profile), a Gaussian atom cloud density distribution with rms width $\sigma$, and we assume these Gaussians are centered on one another. We also

assume a Gaussian distribution of velocities and corresponding Doppler detunings. The deadtime between the mirror pulses is set to be equal to the duration of a $\pi$-pulse. The simulation incorporates four experimental parameters: The Rabi frequency at the center of the cloud ($\Omega_0$), the atom cloud's Doppler detuning spread ($\Delta\nu$), the overall laser detuning ($\delta_0$), and the ratio of the interferometer beam's size to the atom cloud's size ($w_0/\sigma$). We solve for the excited state population after the final beamsplitter pulse for an atom which sees an interferometer beam with detuning $\delta = \delta_p + \delta_0$—where $\delta_p$ corresponds to the Doppler detuning for a particular $p$—and Rabi frequency $\Omega$, $\rho_{ee}[\delta, \Omega, \phi_b]$, where $\phi_b$ is the phase of the final beamsplitter pulse. We solve for $\rho_{ee}$ over a range of $\delta$ and $\Omega$ and then average over these values in a way that is weighted with the expected atom spatial and Doppler detuning distributions:

$$
\begin{aligned}
\bar{\rho}_{ee}(\phi_b) &= \int_{-\infty}^{\infty} d\delta_p \Big(\frac{1}{2\pi\Delta\nu^2}\Big)^{1/2} e^{-\frac{1}{2\Delta\nu^2}\delta_p^2} \int_0^{\infty} 2\pi r dr \Big(\frac{1}{2\pi\sigma^2}\Big)^{2/2} e^{-\frac{1}{2\sigma^2}r^2} \rho_{ee}\Big[\delta_p + \delta_0, \Omega_0 e^{-\frac{1}{w_0^2}r^2}, \phi_b\Big] \\
&= \int_{-\infty}^{\infty} d\delta_p \Big(\frac{1}{2\pi\Delta\nu^2}\Big)^{1/2} e^{-\frac{1}{2\Delta\nu^2}\delta_p^2} \int_0^{\infty} r' dr' e^{-\frac{1}{2}(r')^2} \rho_{ee}\Big[\delta_p + \delta_0, \Omega_0 e^{-\frac{1}{(w_0/\sigma)^2}r'^2}, \phi_b\Big]
\end{aligned}
$$

The inhomogeneity of the Rabi frequency across the atom cloud is captured by the 2D spatial integral over the atom cloud profile, noting that the Rabi frequency scales as the electric field and therefore as square root of the interferometer beam intensity. We simplify this as a 1D integral over a radial coordinate $r$, which can be simplified further by writing it in terms of the transformed coordinate $r' = r/\sigma$. We determine $\bar{\rho}_{ee}(\phi_b)$ for 11 different values of $\bar{\rho}_{ee}(\phi_b)$ and fit the results to an interference fringe of the form $\frac{1}{2}\left(1 + v\cos[\Delta\phi + \phi_b]\right)$. This allows the interferometer visibility $v$ and phase $\Delta\phi$ to be extracted from the simulation. The value of $\rho_{ee}[\delta, \Omega, \phi_b]$ is constructed for different values of $\delta$ and $\Omega$ using analytic solutions to the optical Bloch equation [9], where unitary transformations are done to account for the modulating laser phase between atom-optics pulses. The Doppler detuning integral above is evaluated as a weighted discrete sum over 61 uniformly spaced detunings between $\pm 4\Delta\nu$. Similarly, the spatial integral is computed over 61 uniformly spaced radial positions from 0 to $4\sigma$, corresponding to 61 Rabi frequency samples. Each $\bar{\rho}_{ee}(\phi_b)$ value is thus derived from $61 \times 61$ sequence simulations. To reduce computation time, the sequence simulations are calculated in parallel on the Northwestern Quest computing cluster.

### B. Determination of Experimental Parameters for Simulations

In this section, we detail the parameter estimation and simulation procedures utilized to model the atom interferometer's performance. $\Omega_0$ and $w_0/\sigma$ are determined from fits to multiple Rabi flops, with errors given by the standard deviation. $\Delta\nu$ is determined from the coherence length measurements of Sec. III, and error in this parameter is determined from uncertainty in the Gaussian fit of $V(\delta d_a)$. We use the expression $\Delta\nu = \frac{2\hbar}{mcx_c} f_0$ to relate the coherence length to the thermal Doppler detuning spread of atoms in the cloud, where $f_0$ is the corresponding frequency of the laser field [8]. $\delta_0$ is nominally zero, with uncertainty determined from experimental uncertainty in the calibration of the frequency of the interferometer beam to the 689 nm resonance. In Figure 3 of the main text, we use $\Delta\nu = 0.88 \pm 0.05$ MHz and $w_0/\sigma = 3.06 \pm 0.36$. For the figure in panel (a), we use $\Omega_0 = 7.10 \pm 0.27$ MHz and scan over $\delta_0$, and for the figure in panel (b), we use $\delta_0 = 0 \pm 100$ kHz, and scan over $\Omega_0$ with a center value at $\Omega_0 = 5.92$ MHz. The center value of $\Omega_0$ for Fig. 3(b) is lower than that of Fig. 3(a) owing to the lower interferometer beam power available at the time the data from panel (b) was collected. In Fig. 3(a), we used a pulse deadtime and $\pi$-pulse duration of 80 ns; in Fig. 3(b), we used 96 ns. To estimate uncertainties in the theory curves of Fig. 3, using these uncertainties in independently measured experimental parameters, we scan over the $3^3 = 27$ different combinations of expected value, upper bound, and lower bound of the relevant parameters. In Fig. 3(a), the three parameters are $\Omega_0$, $\Delta\nu$, and $w_0/\sigma$, and in panel (b) the scanned parameters are $\Delta\nu$, $w_0/\sigma$, and $\delta$. The shaded region of the plot in Figure 3 indicates the subsequent minimum and maximum values for the visibility and phase. This method provides a conservative estimation of the uncertainty in our theoretical predictions. The Rabi frequency error plotted along the horizontal axis of Fig. 3(b) is determined experimentally by adjusting the power of the interferometer beam while keeping the pulse durations constant. The simulation results of Figures 4(b-d) of the main text and Fig. 6 of Sec. VII of the supplement use the same expected values of parameters as in Fig. 3(a) of the main text.

## VI. CLOSED-LOOP OPTIMIZATION

In this section, we provide further details on the closed-loop optimization. As described in the main text, we reduce the dimensionality of the $N = 8$ optimization problem to a 2 dimensional problem by writing out the 8-pulse sequences in terms of two parameters, $\phi_1$ and $\phi_2$, where the sequence of 8 pulses is of the form $(\phi_1, \phi_2, \phi_2 + \pi, \phi_1 + \pi, \phi_1 + \pi, \phi_2 +$

$\pi, \phi_2, \phi_1$), which is chosen to suppress the build-up of spurious interference from spontaneous emission. We solve the 2-dimensional optimization problem at $L = 256$ loops by defining a fitness function $f(\phi_1, \phi_2) = v\cos^4(\Delta\phi_0/2)$, where $v$ is the experimentally determined interferometer visibility, and $\Delta\phi_0$ is the deviation of the interferometer phase from its expected value (for all combinations of $\phi_1$ and $\phi_2$, the expected value is zero). The closed-loop optimization shown in Fig. 4(b) of the main text is fully automated. Sampling the fitness function consists of scanning the final beamsplitter phase $\phi_b$ over 11 points from 0 to $2\pi$, then fitting the excited state population to a sinusoidal fringe to extract $v$ and $\Delta\phi_0$, which are used to determine the fitness value. We perform momentum-based gradient ascent on $f$, in which a momentum term is introduced to add robustness to shot-to-shot fluctuations in the measurements from technical noise [10], to optimize the values of $\phi_1$ and $\phi_2$. An initial $\phi_i^0$ for $i = 1, 2$ is sampled, then the subsequent points $\phi_i^k$ are determined according to the equation

$$\phi_i^{k+1} = \phi_i^k + \frac{\gamma g_i^k}{\sqrt{(\gamma g_i^k/\delta\phi)^2 + 1}} + p_i^k,$$

where the gradient of $f$ at step $k$ about the two dimensions is approximated by the expressions $g_1^k$ and $g_2^k$ defined as

$$g_1^k = \frac{f(\phi_1^k + \delta\phi, \phi_2^k) - f(\phi_1^k, \phi_2^k)}{\delta\phi} \qquad g_2^k = \frac{f(\phi_1^k, \phi_2^k + \delta\phi) - f(\phi_1^k, \phi_2^k)}{\delta\phi}$$

We attenuate the gradient step by a factor of $\sqrt{(\gamma g_i^k/\delta\phi)^2 + 1}$ to prevent sharp increases in visibility from causing the optimizer to overshoot when nearing an optimal point. Our particular choice of attenuation factor limits the maximum step size to $\delta\phi$. Afterwards, the 'momentum' term is updated according to

$$p_i^{k+1} = \gamma_p \left( p_i^k + \frac{\gamma g_i^k}{\sqrt{(\gamma g_i^k/\delta\phi)^2 + 1}} \right)$$

with an initial value of $p_i^0 = 0$. We set the 'learning rate' $\gamma = 0.001$, the increment used to evaluate gradients to $\delta\phi = 0.002 \times 2\pi$, and the 'friction coefficient' $\gamma_p = 0.4$. The friction is used to determine how much influence previous gradients have on the current step [10]. A higher value of $\gamma_p$ means momentum persists longer and averages out more noise at the risk of overshooting a maximum. For the example shown in Fig. 4(b) of the main text, we find that this gradient-based optimizer converges after approximately 25 steps.

## VII. CUMULATIVE SPONTANEOUS EMISSION PHASE: DETAILS OF BLOCH SPHERE CONSTRUCTION AND SIMULATIONS

Here we provide further details on the construction of the Bloch spheres depicted in Fig. 4(a) of the main text. For simplicity of visualization, we assume no laser detuning and Rabi frequency error, and that the probability of spontaneous decay per unit time is independent of the excited state population (note that these assumptions are not made in our OBE simulations of the experiment). As shown in Fig. 4(a)(i-iii), after the first pulse is applied, the atomic state is rotated counter-clockwise, and the decayed atoms are distributed on a semi-circular arc producing a non-zero phase shift if averaged over the distribution. During the next pulse, the arc is rotated back through the ground state (i.e, the south pole), causing the atoms that decayed during the first pulse to overlap on the Bloch sphere with the atoms that decayed during the second pulse. If this process of alternating phases is continued for the length of the pulse sequence, the final distribution of the atoms will be a single semi-circular arc containing all spontaneously emitted atoms, producing a cumulative non-zero phase shift that can dominate the interferometer. In comparison, consider a sequence in which all pulse phases are the same, rather than alternating with a $\pm\pi/2$ phase as for 4(a)(i-iii). In this example, the arc formed from the first pulse will rotate through the excited state (i.e, the north pole) and will not overlap with the newly created arc from the second pulse. Because the arcs are opposite to one another, the cumulative phase averages to zero.

To prevent the buildup of a cumulative phase due to spontaneous emission, various constraints can be applied. As described in the main text, for our closed-loop optimization, we explored a specific parameter space defined by repeated groups of $N = 8$ pulses that follow the phase pattern $\phi_1$, $\phi_2$, $\phi_2 + \pi$, $\phi_1 + \pi$, $\phi_1 + \pi$, $\phi_2 + \pi$, $\phi_2$, $\phi_1$, where $\phi_1$ and $\phi_2$ can range between 0 and $2\pi$. The arc generated by the first pulse is counterbalanced by an arc opposite in phase from the fifth pulse. Similarly, the arcs from the second, third, and fourth pulses are cancelled by the arcs from

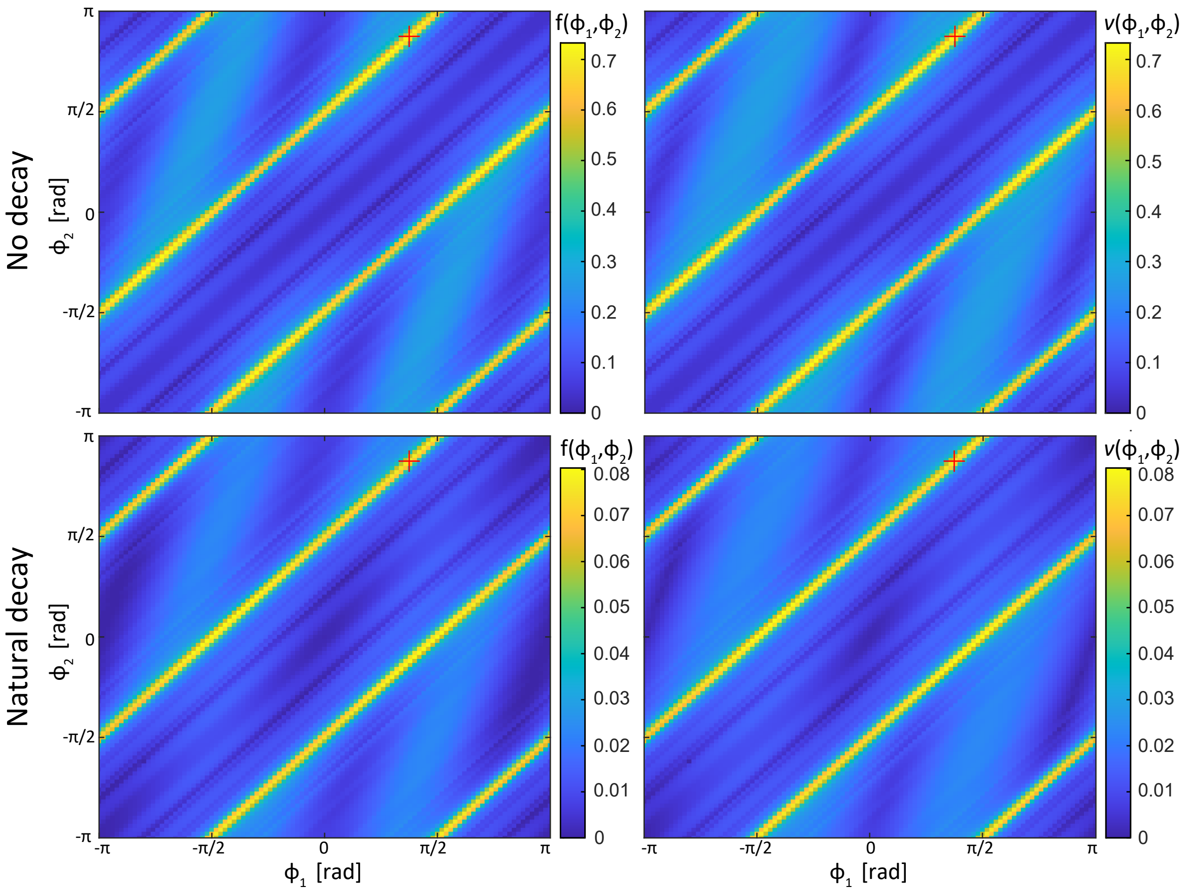


FIG. 6. Simulation results for the $\phi_1$, $\phi_2$, $\phi_2+\pi$, $\phi_1+\pi$, $\phi_1+\pi$, $\phi_2+\pi$, $\phi_2$, $\phi_1$ sequence with 504 loops. Top row: the fitness function $f$ and visibility $v$ result with zero spontaneous decay rate. Bottom row: the fitness function and visibility result with the natural spontaneous decay rate of the $^3P_1$ state included. The "+" indicates the location of the open-loop-optimized sequence shown in Fig. 2 of the main text.

the sixth, seventh, and eighth pulses, respectively. This parametrization was chosen also because it includes some of the best performing sequences found through the open-loop optimization.

Simulations of the fitness function value and interferometer visibility in this parameter space are shown in Fig. 6, both with spontaneous emission occurring at the natural rate and with spontaneous emission artificially omitted. The overall form of the fitness function as a function of $\phi_1$ and $\phi_2$ remains unchanged whether or not spontaneous emission is included in the simulation. The shape of the fitness function matches the interferometer visibility in both cases, recalling that we define the fitness as $f = v\cos[\Delta\phi_0/2]^4$. Unlike the alternating $\pm\pi/2$ sequence, the fitness and visibility within this parameter space do not exhibit any anomalous peaks in visibility associated with spontaneous emission. The overall visibility difference between simulations with and without spontaneous emission aligns with the expected scaling of visibility falloff when atoms that spontaneously emit are considered to form an incoherent background. When the decayed atoms are treated as an incoherent background, the visibility is expected to scale approximately as $v \propto e^{-\gamma T_{\mathrm{seq}}/2}$ where $T_{\mathrm{seq}}$ is the duration of the interferometer sequence, and $\gamma$ is the natural decay rate of the $^3P_1$ state ($\gamma \approx 2\pi \times 7.4$ kHz) [11]. The simulation results shown in Fig. 6 are for a 504-loop sequence with 80 ns $\pi$-pulses and an 80 ns deadtime between pulses, resulting in a total sequence duration of $T_{\mathrm{seq}} \approx 504 \times 2 \times 80$ ns. The expected visibility reduction factor is $e^{-\gamma T_{\mathrm{seq}}/2} \approx 0.15$, which approximately aligns with the overall visibility suppression observed between the simulation including spontaneous emission and the one without it. These results therefore indicate that parameterizing the $N = 8$ optimization problem in this way suppresses the cumulative phase buildup. We note that the spontaneous emission limit curve shown in Fig. 2(c) of the main text uses the approximated visibility reduction factor described above, and therefore does not account for visibility buildup arising from the cumulative phase effect—noting that interferometer sequences that do have such a visiblity buildup do not immediately appear to be useful for measuring oscillating signals.

[1] J. Rudolph, T. Wilkason, M. Nantel, H. Swan, C. M. Holland, Y. Jiang, B. E. Garber, S. P. Carman, and J. M. Hogan, Large momentum transfer clock atom interferometry on the 689 nm intercombination line of strontium, Phys. Rev. Lett. **124**, 083604 (2020).
[2] G. T. Genov, D. Schraft, N. V. Vitanov, and T. Halfmann, Arbitrarily accurate pulse sequences for robust dynamical decoupling, Physical Review Letters **118** (2017).
[3] J. M. Hogan, D. M. S. Johnson, and M. A. Kasevich, Light-pulse atom interferometry (2008), arXiv:0806.3261 [physics.atom-ph].
[4] K. Bongs, R. Launay, and M. A. Kasevich, High-order inertial phase shifts for time-domain atom interferometers, Applied Physics B **84**, 599 (2006).
[5] P. W. Graham, J. M. Hogan, M. A. Kasevich, and S. Rajendran, New method for gravitational wave detection with atomic sensors, Physical Review Letters **110**, 10.1103/physrevlett.110.171102 (2013).
[6] P. Asenbaum, C. Overstreet, and M. A. Kasevich, Matter waves and clocks do not observe uniform gravitational fields, Physica Scripta **99**, 046103 (2024).
[7] P. I. Frazier, A tutorial on bayesian optimization (2018), arXiv:1807.02811.
[8] L. P. Parazzoli, A. M. Hankin, and G. W. Biedermann, Observation of free-space single-atom matterwave interference, Physical Review Letter **109**, 1 (2012).
[9] H.-R. Noh and W. Jhe, Analytic solutions of the optical bloch equations, Optics Communications **283**, 2353 (2010).
[10] B. T. Polyak, *Introduction to optimization* (New York, Optimization Software, 1987).
[11] H. J. Metcalf and P. Van der Straten, *Laser cooling and trapping* (Springer Science & Business Media, 1999).
